# Supplementary material for: Explaining Reinforcement Learning Policies through Counterfactual Trajectories
Source: arXiv:2201.12462 source file (2022-03-19)
Supplement: Supplementary file 1 [file 7_mathappendix.tex]

\subsection{Theoretical Intuition [v2]}

In order to craft useful explanations for reinforcement learning applications, we first discuss what components can be explained.
A reinforcement learning agent observes a \textbf{state} from its environment and takes an \textbf{action} according to its \textbf{policy} to obtain some future \textbf{reward} \cn. 
Many of these components can be explained through explainable AI methods \cn. 
For example, explanations in autonomous vehicles can cover the its interpretation of the sensory data (state), the controls it operates (actions), the destination (reward), and how it decides its path (policy).
In this work, we focus on explaining the policy because it is the most impactful component in interacting with other agents and humans.
In reference to behavior cloning, we call the policy we seek to explain the \textbf{behavior policy} \cn.
In parallel behavior cloning, a human would attempt to mentally clone the behavior policy in order to understand it similarly to how an algorithm would learn the behavior policy from data.
In practice, reinforcement learning environments are not static and may observe distribution shift.
We distinguish three types of environment distributions: the train environment, explain environment, and test environment.
In the train environment, data is collected and a behavior policy is learned. 
In the explain environment, we generated explanations to understand the behavior policy.

In the test environment, we evaluate the behavior policy and test generalization. The probability of a trajectory $\tau$ in the test environment collected by running the behavioral policy $\theta$ is
\begin{align}
p^{\text{test}}(\tau | \theta) &= p_0^{\text{test}}(s_0) \prod_{t=1}^{T} \pi_\theta(a_{t-1} | s_{t-1}) p^{\text{test}}(s_{t} | s_{t-1}, a_{t-1})
\end{align}

Intuitively explanation videos will be more informative the closer the distribution of explanatory videos the agent sees is to the distribution of trajectories the agent will see at test time. As a result, we aim to minimize the KL divergence between the test-time visitation distribution and the distribution shown in the explanations. 

\begin{align}
    \min_{\phi} KL(p^{\text{test}}(\tau | \theta) || p^{\text{expl}}(\tau | \theta, \phi)),
\end{align}

where $\phi$ parameterizes the method we use to generate the explanations, as discussed below.

\section{Counterfactual States [v2]}
It is often desirable to evaluate a behavior policy in states that are not typically observed in the training data.
We call these \textbf{counterfactual states} because we can frame it as a counterfactual question: "what would the behavior policy do if it instead navigated to this state?"
To formulate this, we use an \textbf{exploration policy} $\phi$ that navigates to the counterfactual state.
The exploration policy starts from an arbitrary state in the training data and takes actions until it reaches a counterfactual state (Figure \ref{fig:cf_states}). 

The explanations we show the user are generated by starting in this counterfactual state and rolling out the behavioral policy for the remainder of the trajectory. This gives us a visitation distribution of 

\begin{align}
p^{\text{expl}}(\tau | \theta, \phi) &= p_0^{\text{expl}}(s_0 | \phi) \prod_{t=1}^{T} \pi_\theta(a_{t-1} | s_{t-1}) p^{\text{train}}(s_{t} | s_{t-1}, a_{t-1}),
\end{align}

where $p_0^{\text{expl}}(s_0 | \phi)$ is the distribution of final states the agent reaches as a result of running the exploration policy for a certain number of timesteps. 

\subsection{Exploration Policy Design}
We'd like our exploration policy $\pi_\phi$ to produce a trajectory distribution which closely matches the test-time distribution. To do this, we first make the assumption that $p^{\text{train}}(s_{t} | s_{t-1}, a_{t-1}) \approx p^{\text{test}}(s_{t} | s_{t-1}, a_{t-1})$. This restricts the applicability of our method to distribution shifts in which we expect minimal dynamics changes, for instance shifts where at test time the agent is placed in a new start state in the environment. With this approximation, we observe that because the explanation visitation distribution and the test visitation distribution use the same policy and dynamics, the ratio of the trajectory probabilities depends solely n the ratio of the start state probabilities.

\begin{align}
    & \min_{\phi} KL(p^{\text{test}}(\tau | \theta) || p^{\text{expl}}(\tau | \theta, \phi)) \\
    &= \min_{\phi} \int p^{\text{test}}(\tau | \theta) \log \left( \frac{p^{\text{test}}(\tau | \theta)}{p^{\text{expl}}(\tau | \theta, \phi)} \right) \\
    &= \min_{\phi} \int p^{\text{test}}(\tau | \theta) \log \left( \frac{p^{\text{test}}(\tau | \theta)}{p^{\text{expl}}(\tau | \theta, \phi)} \right) \\
    &= \min_{\phi} \int p^{\text{test}}(\tau | \theta) \log \left( \frac{p_0^{\text{test}}(s_0) \prod_{t=1}^{T} \pi_\theta(a_{t-1} | s_{t-1}) p^{\text{test}}(s_{t} | s_{t-1}, a_{t-1})}{p_0^{\text{expl}}(s_0 | \phi) \prod_{t=1}^{T} \pi_\theta(a_{t-1} | s_{t-1}) p^{\text{train}}(s_{t} | s_{t-1}, a_{t-1})} \right) \\
    &= \min_{\phi} \int p^{\text{test}}(\tau | \theta) \log \left( \frac{p_0^{\text{test}}(s_0) \prod_{t=1}^{T}  p^{\text{test}}(s_{t} | s_{t-1}, a_{t-1})}{p_0^{\text{expl}}(s_0 | \phi) \prod_{t=1}^{T} p^{\text{train}}(s_{t} | s_{t-1}, a_{t-1})} \right) \\
    &= \min_{\phi} \int p^{\text{test}}(\tau | \theta) \left[ \log \left( \frac{p_0^{\text{test}}(s_0) }{p_0^{\text{expl}}(s_0 | \phi) } \right) + \log \left( \frac{\prod_{t=1}^{T}  p^{\text{test}}(s_{t} | s_{t-1}, a_{t-1})}{\prod_{t=1}^{T} p^{\text{train}}(s_{t} | s_{t-1}, a_{t-1})} \right) \right] \\
    \intertext{The rightmost term has no dependence on $\phi$, so it can be removed. \jf{Not sure we can assume this} \ow{Why not, isn't this just the dynamics? But I agree something fishy is going on here, b/c this seems to suggest that our method works fine no matter how crazily different the train/test dynamics are, which is intuitively untrue.} \ow{After talking with some people, I think this is mathematically true. We're sampling $\tau$ from the test distribution, and computing the probability of the entire trajectory under the test distribution vs the expl distribution. The probability of a trajectory is the product of a bunch of terms, and $\phi$ only affects the first. I think we could use this to argue that our explanation will only be useful (i.e. the KL between test and expl will only be low) if the dynamics match. However, we don't need pay attention to this while choosing $\phi$.}}
    &= \min_{\phi} \int p^{\text{test}}(\tau | \theta) \left[ \log \left( \frac{p_0^{\text{test}}(s_0) }{p_0^{\text{expl}}(s_0 | \phi) } \right) \right] \\
    \intertext{We can upper-bound the probability of a trajectory with the probability of its start state. \ow{I'm kind of suspicious since it's not a tight upper bound.}}
    &\leq \min_{\phi} \int p_0^{\text{test}}(s_0 ) \log \left( \frac{p_0^{\text{test}}(s_0)}{p_0^{\text{expl}}(s_0 | \phi)} \right) \\
    &= \min_{\phi} KL(p_0^{\text{test}}(s_0) || p_0^{\text{expl}}(s_0 | \phi))
\end{align}

\ks{I think the math looks right, the reason your minimization only depends on the initial state distribution is because that is the only thing you are changing, i.e. if you were also trying to approximate the test-time state transition probability, then the last term would depend on $\phi$ and would not disappear. So basically, you are simplifying things by assuming that the dynamics do not change, then the main difference between the train and test trajectories will be the initial states, because once you start in a state, the rest will be the same. }

Intuitively, this means that our exploration policy should aim to visit the start states we expect to see in the test environment. Practically speaking, however, we rarely know $p_0^{\text{expl}}(s_0 | \phi)$ before encountering the test-time distribution, so we are unable to choose our exploration policy $\phi$ by directly minimizing this equation. Instead, we must choose a prior distribution for the test start distribution and optimize this instead. If we have domain knowledge of the distribution shift we expect to see in the environment, then we could construct a target exploration distribution which reflects this.  In this work, however, we make the simplifying assumption that we have a uniform distribution over start states.

In this work, we use manually hard-coded exploration policies to achieve a uniform distribution over states, which results in the minimum possible KL divergence of 0. Future work in environments where this is not possible could expand on this by directly estimating the KL divergence and optimizing $\phi$ to minimize it.
\ks{That sounded like a cop out, maybe soften it by arguing that the main focus of this work is in showing this works with humans}

\begin{figure}
    \centering
    \caption{Counterfactual States}
    \label{fig:cf_states}
\end{figure}

\section{Preliminaries [v1]}
In order to craft useful explanations for reinforcement learning applications, we first discuss what components can be explained.
A reinforcement learning agent observes a \textbf{state} from its environment and takes an \textbf{action} according to its \textbf{policy} to obtain some future \textbf{reward} \cn. 
Many of these components can be explained through explainable AI methods \cn. 
For example, explanations in autonomous vehicles can cover the its interpretation of the sensory data (state), the controls it operates (actions), the destination (reward), and how it decides its path (policy).
In this work, we focus on explaining the policy because it is the most impactful component in interacting with other agents and humans.
In reference to behavior cloning, we call the policy we seek to explain the \textbf{behavior policy} \cn.
In parallel behavior cloning, a human would attempt to mentally clone the behavior policy in order to understand it similarly to how an algorithm would learn the behavior policy from data.
In practice, reinforcement learning environments are not static and may observe distribution shift.
We distinguish three types of environment distributions: the train environment, explain environment, and test environment.
In the train environment, data is collected and a behavior policy is learned. 
In the explain environment, we generated explanations to understand the behavior policy. 
In the test environment, we evaluate the behavior policy and test generalization.
\begin{align}
p(\tau_{0:t} | \theta) &= p_0(s_0) \prod_{t'=1}^{t} \pi_\theta(a_{t'-1} | s_{t'-1}) p(s_{t'} | s_{t'-1}, a_{t'-1})
% \\p(s | \theta) &= \sum_{t=0}^{T} p(s_t = s| \theta)
\end{align}

% \begin{enumerate}
% \item[(1)] The probability of reaching state $s_t$ with the behavior policy $\pi_\theta$.
% \item[(2)] The probability distribution over states given our parameters $\theta$.
% \end{enumerate}

\section{Counterfactual States [v1]}
It is often desirable to evaluate a behavior policy in states that are not typically observed in the training data.
We call these \textbf{counterfactual states} because we can frame it as a counterfactual question: "what would the behavior policy do if it instead navigated to this state?"
To formulate this, we use an \textbf{exploration policy} that navigates to the counterfactual state.
The exploration policy starts from an arbitrary state in the training data and takes actions until it reaches a counterfactual state (Figure \ref{fig:cf_states}).
% \begin{align*}
% p(s_t | \theta) &= p_0(s_0) \prod_{t'=1}^{t} \pi_\theta(a_{t'-1} | s_{t'-1}) p(s_{t'} | s_{t'-1}, a_{t'-1})
% \\p_k(s_t | \theta, \phi) &= p(s_k | \theta) \prod_{t'=k+1}^{t} \pi_\phi(a_{t'-1} | s_{t'-1}) p(s_{t'} | s_{t'-1}, a_{t'-1})
% \\p(s_t | \theta, \phi) &= \sum_{k=0}^{t-1} p_k(s_t | \theta, \phi)
% \\p(s | \theta, \phi) &= \sum_{t=1}^{T} p(s_t | \theta, \phi)
% \end{align*}
\begin{align}
p(\tau_{0:t+k} | \theta, \phi) &= p(\tau_{0:t} | \theta) \prod_{t'=t+1}^{t+k} \pi_\phi(a_{t'-1} | s_{t'-1}) p(s_{t'} | s_{t'-1}, a_{t'-1})
\\p(\tau_{0:T} | \theta, \phi) &= \underset{t,k}{\mathbb{E}} \Big [ p(\tau_{0:t+k} | \theta, \phi) \prod_{t'=t+k+1}^{T} \pi_\theta(a_{t'-1} | s_{t'-1}) p(s_{t'} | s_{t'-1}, a_{t'-1}) \Big ]
\end{align}
% \begin{enumerate}
% \item[(3)] The probability of reaching counterfactual state $s_{t,k}$ with the behavior policy $\pi_\theta$ for $t$ steps and exploration policy $\pi_\phi$ for $k$ steps.
% \item[(4)] The probability distribution over counterfactual states given our parameters $\theta$, $\phi$.
% \end{enumerate}
The values of $t$ and $k$ can potentially be sampled from sophisticated distributions, but in this work we uniformly sample $t \in [0, ..., T-k]$ and a fixed $k$ depending on the environment and exploration policy.

\subsection{Exploration Policy Design}
We'd like our exploration policy $\pi_\phi$ to produce a trajectory in the train environment that is maximally informative of the behavior policy $\pi_\theta$ in the test environment.
To do so, we can maximize the mutual information between the trajectory distributions in the train and test environments.
\begin{align*}
\max_\phi I(p_\text{train}(\tau | \theta, \phi), p_\text{test}(\tau | \theta))
\end{align*}
Where $p_\text{train}(\tau | \theta, \phi)$ is the counterfactual trajectory distribution in the train environment and $p_\text{test}(\tau | \theta)$ is the trajectory distribution following policy $\pi_\theta$ in the test environment.

Since it's not always the case where we can sample trajectories in the test environment, we can use a pessimistic lower bound and maximize the entropy of $p_\text{train}(\tau | \theta, \phi)$.
\begin{align*}
I(p_\text{train}(\tau | \theta, \phi)), p_\text{test}(s | \theta))
&= H(p_\text{train}(\tau | \theta, \phi)) - H(p_\text{train}(\tau | \theta, \phi) | p_\text{test}(s | \theta))
\\&\leq H(p_\text{train}(\tau | \theta, \phi))
\end{align*}
\ow{Feels sketchy to me? If we drop the 2nd term, we're dropping everything that requires that the train distribution know anything about the test distribution, so it seems hard to say we're still maximizing mutual info.}

Intuitively, by increasing the entropy of counterfactual trajectories we are hoping that we cover more information about the test environment.

======= ignore notes below =======

However, it's not always the case where we have information of the state distribution in the test environment.
Therefore, we can use a pessimistic upper bound and just maximize the entropy of $p_\text{train}(s | \theta, \phi)$.

\begin{align*}
I(p_\text{train}(s | \theta, \phi), p_\text{test}(s | \theta))
&= H(p_\text{train}(s | \theta, \phi)) - H(p_\text{train}(s | \theta, \phi) | p_\text{test}(s | \theta))
% \\&= H(p_\text{test}(s | \theta)) - H(p_\text{test}(s | \theta) | p_\text{train}(s | \theta, \phi))
\\&\leq H(p_\text{train}(s | \theta, \phi))
\end{align*}
Intuitively, by increasing the entropy of counterfactual states $H(p_\text{train}(s | \theta, \phi))$ we are maximally covering the state space and hoping that the test environment distribution is within. By minimizing $H(p_\text{train}(s | \theta, \phi) | p_\text{test}(s | \theta))$, the counterfactual states are encouraged to converge when we know the test state visitation distribution $p_\text{test}(s | \theta)$.

If we instead had ground truth data of our agent in the test environment, we could use the reverse mutual information form to directly optimize the exploration policy.
\begin{align*}
I(p_\text{train}(s | \theta, \phi), p_\text{test}(s | \theta))
&= H(p_\text{test}(s | \theta)) - H(p_\text{test}(s | \theta) | p_\text{train}(s | \theta, \phi))
\end{align*}

In this work, however, we use heuristic policies to approximate the optimal exploration policy.

Lastly, one could consider a KL objective
\begin{align}
\min_\phi KL(p_\text{train}(s | \theta, \phi) \| p_\text{test}(s | \theta))
\end{align}

\subsection{User Evaluation}
When working with RL agents, it is often necessary for humans to understand their behavior. We call this task policy understanding. First, we roll out a trained behavior policy in the training environment $\pi_\theta$ to produce a dataset $D_\text{train}$. Then, a user observes trajectory samples $\tau \in D_\text{train}$ and constructs a mental model of the policy $\pi_{\theta'}$. Lastly, the user's mental model is evaluated by comparing it to rollouts of the behavior policy in the test environment.
One can formulate the user's objective as the following:
\begin{align*}
\min_{\theta'} \underset{s, a \sim \pi_{\theta}}{D_\text{KL}} (\pi_{\theta}(s, a) \| \pi_{\theta'}(s, a))
\end{align*}

Behavior cloning objective:
\begin{align*}
\min_{\theta'} \underset{s, a \sim \pi_{\theta}}{\mathbb{E}}[-\log \pi_{\theta'}(a = \pi_{\theta}(a|s)|s)]
\end{align*}
